# Supplementary material for: 10^(10^6) Worlds and Beyond: Efficient Representation and Processing of Incomplete Information
Source: arXiv:cs/0606075 source file (2008-02-13)
Supplement: Supplementary file 1 [file appendix.tex]

%-------------------------------
\section{Appendix}

\begin{figure*}[htbp]
  \centering

\parbox{8.5cm}{
\begin{align}\label{def:ext}
  \textsf{ext} (C,A_i,B) = \{&(A_1:a_1,\ldots,A_n:a_n,B:a_i)\mid\\
  &(A_1:a_1\ldots,A_n:a_n)\in C\} \nonumber
\end{align}}
\hfill
\parbox{8.5cm}{
\begin{align}\label{rule:copy}
  \frac{C\in\mathcal{C}\wedge R.t.A\in\mathcal{S}(C)\wedge P.t.A\not\in\mathcal{S}(C)}%
  {C:=\textsf{ext}(C, R.t.A, P.t.A)}
\end{align}}
\parbox{8.5cm}{
\begin{align}\label{rule:constcond}
\sigma_{A \theta c} R:\;
  &\frac{C\in\mathcal{C}\wedge P.t.A\in\mathcal{S}(C)\wedge
  t_C\in C\wedge \neg(t_C.(P.t.A) \,\theta\, \textsf{c})}%
  {t_C.(P.t.*) := \bot}
\end{align}}
\hfill
\parbox{8.5cm}{
\begin{align}
\sigma_{A \theta B} R:\;
  &C\in\mathcal{C}\wedge P.t.A, P.t.B\in\mathcal{S}(C)\wedge \nonumber\\
  &\frac{t_C\in C\wedge \neg(t_C.(P.t.A) \,\theta\, t_C.(P.t.B))}%
  {t_C.(P.t.*) := \bot} \label{rule:joincond1}
\end{align}}

\parbox{8.5cm}{
\begin{align}
merge: &
  \frac{C_1,C_2\in\mathcal{C}\wedge P.t.A\in\mathcal{S}(C_1)\wedge P.t.B\in\mathcal{S}(C_2)}%
  {\mathcal{C}:= \mathcal{C}-\{C_1,C_2\} \cup(C_1\times C_2)}
  \label{rule:joincond2}
\end{align}
}
\hfill
\parbox{8.5cm}{
\begin{align}\label{rule:decomposition}
decomp: &
  \frac{C\in\mathcal{C}\wedge C=C_1\times C_2}%
  {\mathcal{C} := \mathcal{C}-\{C\}\cup\{C_1,C_2\}}
\end{align}
}

\parbox{8.5cm}{
\begin{align}
  &C_1, C_2\in\mathcal{C}\wedge \nonumber\\
cl1:
  &\frac{X.A\in\mathcal{S}(C_1)\wedge X.B\in\mathcal{S}(C_2)\wedge \pi_{X.A}(C_1)=\{\bot\}}%
  {C_2:=\pi_{\mathcal{S}(C_2)-\{X.B\}}(C_2)} \label{rule:clean1}
\end{align}}
\hfill
\parbox{8.5cm}{
\begin{align}
  &C\in\mathcal{C}\wedge X.A\in\mathcal{S}(C)\wedge \nonumber\\
cl2:
  &\frac{\pi_{X.A}(C)=\{\bot\} \wedge\forall C'\in\mathcal{C}(X.B\not\in\mathcal{S}(C'))}%
  {C:=\pi_{\mathcal{S}(C)-\{X.A\}}(C)} \label{rule:clean2}
\end{align}}

\parbox{8.5cm}{
\begin{align}
\pi_U(R):
  &\frac{C\in\mathcal{C}\wedge R.t.A\in\mathcal{S}(C)\wedge A\in U \wedge P.t.A\not\in\mathcal{S}(C)}%
  {C:=\textsf{ext}(C, R.t.A, P.t.A)}\label{rule:proj1}
\end{align}}
\hfill
\parbox{8.5cm}{
\begin{align}
  &C\in\mathcal{C}\wedge X.A,X.B\in\mathcal{S}(C)\wedge \nonumber\\
cl3:
  &\frac{t_C\in C\wedge t_C.X.A=\bot\wedge t_C.X.B\not=\bot}%
  {t_C.X.B:=\bot} \label{rule:proj2}
\end{align}}

\parbox{8.5cm}{
\begin{align}
R \times S:
  &\frac{C\in\mathcal{C}\wedge R.t_i.A\in\mathcal{S}(C)\wedge j\leq|S|\wedge T.(t_i,t_j).A\not\in\mathcal{S}(C)}%
  { C := \textsf{ext}(C, R.t_i.A, T.(t_i,t_j).A)} \label{rule:prod1}
\end{align}}
\hfill
\parbox{8.5cm}{
\begin{align}
R \times S:
  &\frac{C\in\mathcal{C}\wedge S.t_j.A\in\mathcal{S}(C)\wedge i\leq|R| \wedge T.(t_i,t_j).A\not\in\mathcal{S}(C)}%
  { C := \textsf{ext}(C, S.t_j.A, T.(t_i,t_j).A)}  \label{rule:prod2}
\end{align}}

\begin{align}
R \cup S:
  &\frac{C\in\mathcal{C}\wedge X.t.A\in\mathcal{S}(C)\wedge (X=R\vee X=P) \wedge T.t.A\not\in\mathcal{S}(C)}%
  {C := \textsf{ext}(C, X.(X.t).A, T.t.A)} \label{rule:union}
\end{align}
\vspace*{-1em}
\caption{Rules for evaluation of relational algebra operations on WSDs.}
\label{fig:operators}
\end{figure*}

%%% Local Variables: 
%%% mode: latex
%%% TeX-master: "paper"
%%% TeX-master: "paper"
%%% End: 
